# Supplementary material for: Droplet deformation and breakup in shear flow of air
Source: arXiv:2005.06240 source file (2020-05-13)
Supplement: Supplementary file 1 [file DropletBreakup_SM.pdf]

# Droplet deformation and breakup in shear flow of air: Supplementary materials

Zhikun Xu (徐志坤), Tianyou Wang (王天友), and Zhizhao Che (车志钊)*

State Key Laboratory of Engines, Tianjin University, Tianjin, 300072, China.

April 22, 2020

## S1. Effect of the number of instantaneous flow fields on the measurements

To characterize the turbulent velocity field for the droplet breakup, many instantaneous velocity fields were obtained, and they were used to calculate the average velocity fields, the shear strength, and the turbulent kinetic energy (TKE). The number of instantaneous velocity fields ($n$) should be large enough to avoid the statistical bias. Our experimental data showed that the maximum velocity, the maximum shear strength, and the maximum TKE in the flow field were not affected by the number of instantaneous velocity fields when $n > 200$, as shown in FIG. S1. Therefore, the number of instantaneous velocity fields used in this study was chosen to be 250–350.

## S2. Procedure for calculating the fragment diameter

The procedure for calculating the fragments diameter is as follows. We firstly removed the background of the raw images by subtracting an image without any droplet. Then the image was binarized based on a threshold, and the holes in the middle of the fragments in the binary image were filled. After that, objects smaller than 10 pixels were removed from the binary image, as they either corresponded to the small fragments of the bag or noise in the image. Then the areas of the fragments in pixel were obtained from the image by region analysis. The diameters of the droplets were firstly calculated from the areas in pixel and then were converted to the real scale by using a scale factor obtained from a calibration image of a ruler. Since the segmentation process takes time, some secondary droplets may have not broken up while the others have already left the field of view. To solve this problem, the fragments were divided into two groups and were measured in different images, as shown in FIG. S2. By dividing them, we could use a large magnification in imaging for a higher resolution, and selected images at the instants when the droplets were well focused. In addition, we repeated each experimental condition about 30 times to get a statistical result to eliminate the influence of errors caused by the experiment operation.

*Corresponding author: chezhizhao@tju.edu.cn

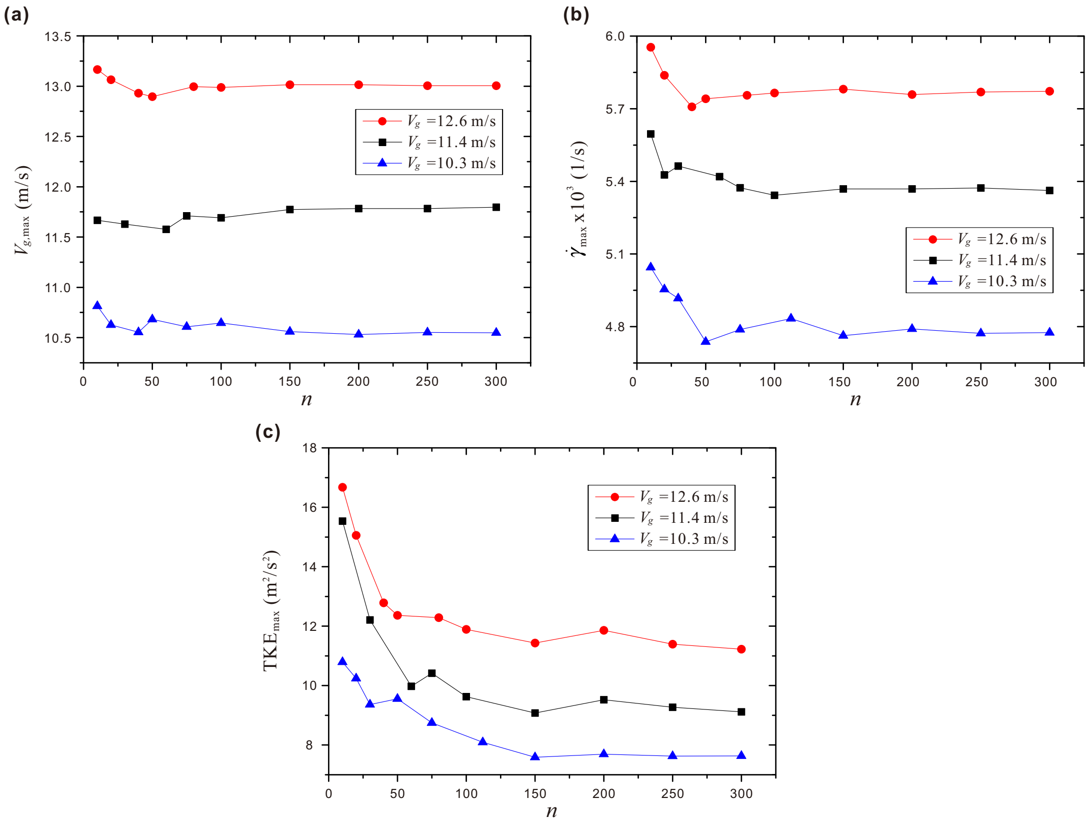


FIG. S1: (a) Maximum velocity ($V_{g,\max}$), (b) maximum shear strength ($\dot{\gamma}_{\max}$), (c) maximum turbulent kinetic energy ($\mathrm{TKE}_{\max}$) under different numbers of instantaneous velocity fields.

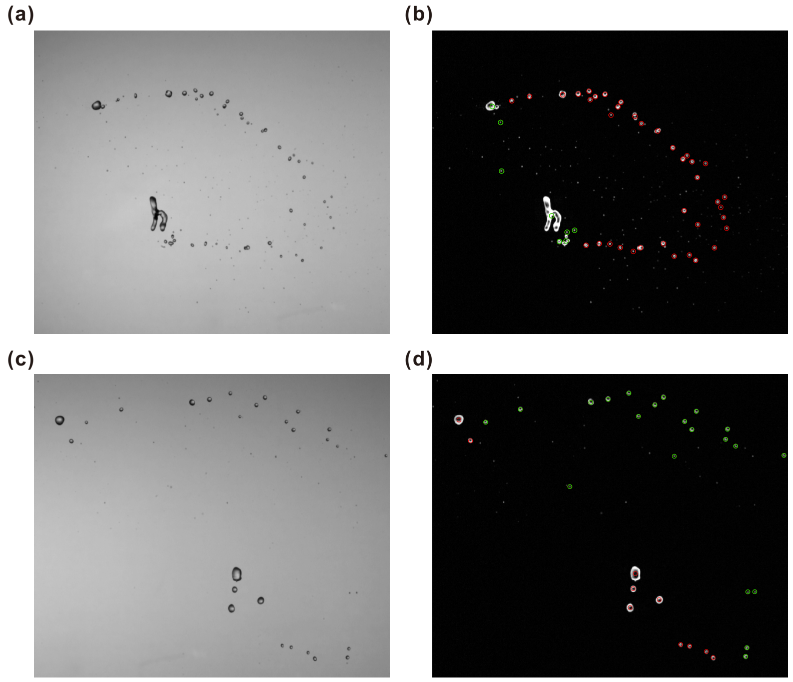


FIG. S2: Measurement of fragments size in different images. (a-b) Raw image and binary image at $t = 25$ ms, mainly for calculating the fragments of the inter-node liquid threads. (c-d) Raw image and binary image at $t = 36.5$ ms, mainly for calculating the fragments of the nodes. The fragments highlighted by the red circles in (b) and (d) include all fragments to consider and are used in the calculation.
